# Supplementary material for: GPTScan: Detecting Logic Vulnerabilities in Smart Contracts by Combining GPT with Program Analysis
Source: arXiv:2308.03314 source file (2024-05-06)
Supplement: Supplementary file 1 [file appendix.tex]

% \newpage
\appendix
%\section*{Appendix}
\subsection{$r$'s Impact on Similarity Measurement}
% \section{}
\label{sec:appendix1}

As illustrated in \mysec\ref{subsec:code_sim}, we introduced the reward factor $r$ to adjust the ordering issue's influence on code similarity.
By calculating all the patch and candidate code's similarities with different $r$, we can evaluate the impact of $r$ on the similarity measurement.
In \myfig\ref{fig:r_sim}, we plot the CDF of similarity with $r$ from 0.15 to 0.95.
As we can see, $r$ has a more significant influence on the similarity when the similarity is low.
Moreover, since we try to minimize false negatives, we need to include more candidate code in the analysis.
As such, we should exclude fewer candidate code that has similarity below the threshold.
According to \myfig\ref{fig:r_sim}, when $r=0.95$, it has the least candidate code with similarity below 0.4.
Therefore, we set 0.95 as the default value of $r$.

\begin{figure}[b!]
	\begin{adjustbox}{center}
		\includegraphics[width=1.0\linewidth]{resources/r_sim_cdf}
	\end{adjustbox}
	\caption{The CDF plot of similarity with different $r$.}
	\label{fig:r_sim}
\end{figure}

% \begin{figure}[h!]
% 	\begin{adjustbox}{center}
% 		\includegraphics[width=1.0\linewidth]{resources/qtum_github}
% 	\end{adjustbox}
% 	\caption{The example of a commit page on Github.}
% 	\label{fig:qtum_commit_exp}
% \end{figure}

% \input{resources/tab/tab_vuln_root_cause}

% \input{resources/tab/tab_patch_outdated}

% \input{resources/tab/tab_target_outdated}
